# Supplementary material for: Digital Twin Catalog: A Large-Scale Photorealistic 3D Object Digital Twin Dataset
Source: arXiv:2504.08541 source file (2025-05-18)
Supplement: Supplementary file 1 [file 6_supp_old.tex]

1. Dataset statistics (3D object category list, object list used in DSLR recording \& aria recordings), more visual examples for 3D objects (PBR), real world recording examples and aria recordings.

2. Benchmark:
    Sparse-view --> LRM (both DSLR and Ego)
    Dense-view --> Neural-PBIR
    Robotic experiment details?   
    Need to spend some time looking at the results for each baseline method, and write a simple result analysis for each baseline. Try to pick up the challenging results that existing work that do not work well and can be surfaced by our evaluation. 
    Need to add shape ground truth evaluation using metrics consistent with the DSLR evaluation. 

3. Dataset processing pipeline description 
    More details on the decisions and results for the dataset generation (alignment) process. 

4. Put a video to highlight digital twin assets. 
    * Fix the color tone mismatch in the current comparison videos. 
    * To show the raw video footage.
